# Supplementary material for: Explainable Deep Reinforcement Learning for Portfolio Management: An Empirical Approach
Source: arXiv:2111.03995 source file (2021-12-18)
Supplement: Supplementary file 1 [file Appendix.tex]

%%%%%%%%%%%%%%%%%%%%%%%%%%%%%%%%%%%%%%%%%%%%%%%%%%%%%%%%
\subsection{Interpretation under Linear Models}

The classical active portfolio management task is composed of 3 steps: 1) feature engineering, 2) empirical modelling and 3) forecasting. 
Each feature is used to predict the return above/below the average level. Interpretation of the task is to understand the relationship between the  weights and each feature so as to understand of source of profit and loss.
Although various models are proposed to derive the best performing  weights,
 linear regression model is mostly accepted and used for it gives the statistical inference as interpretation to the linear relationship between the  weights and features. Specifically for weights, it is assumed to be the combination of equal weight plus a linear combination of features. 
 $\bm{w}(t) = c \cdot \bm{f}(t) + \frac{1}{N}$, $c > 0$
 
 \begin{itemize}
     \item Feature Engineering: Suppose we have K features, and each feature vector is standardized \footnote{Standardization: Given vector $\bm{x}\in \mathbb{R}^N$, ~\text{after standardization}, $\bm{x}_i = \frac{\bm{x}_i - \overline{\bm{x}}}{\sigma(\bm{x})}$ }
     Under liner model, K features are combined as a integrated feature with linear model to derive a weight vector so as to maximize the return.
\begin{equation}
    \begin{split}
        \alpha(t) &= (N-1)\cdot \delta(\bm{w}_i(t))\sigma(\bm{r}_i(t))\\
        &=(N-1)\cdot c^2 \rho(\bm{f}_i(t), \bm{r}_i(t))
        \cdot \sigma(\bm{r}_i(t))
    \end{split}
\end{equation}
Therefore, the return is proportional to the correlation coefficient between $\bm{f}(t)$ and $\bm{r}(t)$. So the linear model aims to combine the K features so as to maximize it. No vector has greater correlation with return vector than itself.
     \item Empirical Modelling: Built cross-sectional linear regression model for the past W time periods.
\begin{equation}
\begin{split}
     \bm{r}(t) &= \beta_0(t) +
\beta_1(t) \bm{f}^1(t) + .. . +\beta_K(t) \bm{f}^K(t)\\&+\epsilon_1(t)\\
\end{split}
\end{equation}
After running the regression, estimated beta $\widehat{\beta}_i(t)$ will be derived. 
     \item Forecasting: Average the estimated regression coefficients of the past W time periods and apply with each feature to derive out forecast.
     \begin{equation}
     \begin{split}
          \widehat{\beta}_i(t) &= \frac{\sum_{j=1}^{W-1} \widehat{\beta}_i(t-j)}{W}, i = 0,...,K, \\
        \widehat{\bm{r}}(t) &= \sum_{i=1}^{K} \widehat{\beta}_{i}(t) \cdot \bm{f}^{i}(t) + \widehat{\beta}_{0}(t)\cdot \bm{1},\\
        \bm{f}(t) &= \sum_{i=1}^{K} \frac{\widehat{\beta}_{i}(t) \cdot \bm{f}^{i}(t)}{\sigma(\sum_{i=1}^{K}\widehat{\beta}_{i}(t) \cdot \bm{f}^{i}(t))}\\  
        \bm{w}(t) &=  c \cdot \bm{f}(t)  + \frac{1}{N}\cdot \bm{1}\\
        \delta(\bm{w}_i(t))&= \frac{Cov(\bm{w}_i(t), \bm{r}_i(t))}{\sigma(\bm{r}_i(t))}\\
        &=  c \cdot \sum_{i=1}^{K}\frac{\widehat{\beta}_i(t)}{\sigma(\sum_{i=1}^{K}\widehat{\beta}_{i}(t) \cdot \bm{f}^{i}(t))} \cdot \delta(\bm{f}^i(t)) \\
        &= c \cdot \bm{\widehat{\beta}}(t) \cdot \bm{\delta}(\bm{f}(t))\\
        &= c \cdot ||\bm{\widehat{\beta}}(t)||_2 \cdot ||\bm{\delta}(\bm{f}(t))||_2 \cdot \cos(\theta)
     \end{split}
     \end{equation}
    where $\theta$ is the angle between vector  $\bm{\widehat{\beta}}(t)$ and $\bm{\delta}(\bm{f}(t))$, and $||\cdot||_2$ is the $\ell_2$ norm.
    Therefore, under linear regression model, the profits at t can be decomposed into inner product of vectors $\bm{\widehat{\beta}}(t)$ and $\bm{\delta}(\bm{f}(t)))$
    %  Therefore, the excess return is linear proportional to the linear correlation coefficient of each feature vector and return vector.
    %  \begin{equation}
    %      \begin{split}
    %          \alpha(t+1) &= C \cdot \Sigma_{i=1}^{i=K} \beta_{i}(t) \rho(\bm{f}^{i}(t), \bm{r}(t+1)) \\
    %              &= C \cdot \bm{\rho}^T(t) \cdot \bm{\beta}(t) \\ 
    %              & = C \cdot ||\bm{\rho}(t)||_{2} \cdot ||\bm{\beta}(t)||_{2} \cdot \cos{(\bm{\rho}(t),\bm{\widehat{\beta}}(t))}
    %      \end{split}
    %  \end{equation}
    %  where C is a positive constant value given the assumption, $\bm{\rho}(t)$, $\bm{\beta}(t)$ is the correlation coefficient vector and the regression coefficient vector at time t. Since $||\bm{\beta}(t)||_2$ is 1 and the norm of the correlation coefficient vector is independent of regression coefficient vector, the excess return at time t + 1 is proportional to the cosine value of vector $\bm{\rho}(t)$ and  $\bm{\beta}(t)$ 
 \end{itemize}

The interpretation under linear regression is then to evaluate the regression coefficient vector's cosine similarity with the linear correlation coefficient vector.

\subsection{Interpretation under Non-linear Models}

For non-linear models, we could adopt a similar approach in Section 3.2. The active weights derived from non-linear models could be taken part into: linear effects and non-linear effects. Similar to the regression coefficient, a marginal effect of model to each feature could be a good metric to represent the sensitivity of each feature vector to the model output. Instead of using a constant $c$, the weight under non-linear model is assumed to be a combination of linear and non-linear combination of features and equal weight.
\begin{equation}
\begin{split}
        \bm{g}((\bm{f}^{1}(t),...,\bm{f}^{K}(t))) &= \bm{l}(t) + \bm{n}(t) + \frac{1}{N} \cdot \bm{1} \\
        \delta{(\bm{g}((\bm{f}^{1}(t),...,\bm{f}^{K}(t))))} &= \delta{(\bm{l}(t))} + \delta{(\bm{n}(t))} \\
        \bm{l}(t) & = \sum_{i=1}^{K}\frac{\partial \bm{g}}{\partial \bm{f}^{i}}\Bigr|_{\bm{f}^{i}(t) = \bm{0}} \cdot \bm{f}^i(t)\\
        \bm{m}(t) &= (\frac{\partial \bm{g}}{\partial \bm{f}^{i}}\Bigr|_{\bm{f}^{i}(t) = \bm{0}})\\
        \delta(\bm{l}(t)) & = \sum_{i=1}^{N} \frac{\partial \bm{g}}{\partial \bm{f}^{i}}\Bigr|_{\bm{f}^{i}(t) = \bm{0}} \cdot \delta(\bm{f}^{i}(t))\\
                          &= \bm{m}(t) \cdot \bm{\delta}(\bm{f}(t))
        % \bm{g}((\bm{f}^{1}(t),...,\bm{f}^{K}(t)))  &\approx  \Sigma_{i=1}^{i=K}\frac{\partial \bm{g}}{\partial \bm{f}^{i}}\Bigr|_{\bm{f}^{i}(t) = \bm{0}} \cdot \bm{f}^i(t) + ~\text{non linear weight}, \\
        % \bm{m}_{i}(t) &= \frac{\frac{\partial \bm{g}}{\partial \bm{f}^{i}}\Bigr|_{\bm{f}^{i}(t) = \bm{0}}_i}{\sqrt{\sum_{i=1}^{i=K} (\frac{\partial \bm{g}}{\partial \bm{f}^{i}}\Bigr|_{\bm{f}^{i}(t) = \bm{0}})^2}},  \\
        % \bm{l}(t) &= \bm{F}(t) \cdot \bm{m}(t), \\
        % \bm{n}(t) &= \frac{\bm{a}(t) - \bm{l}(t)}{\sigma(\bm{a}(t) - \bm{l}(t))}。
\end{split}
\end{equation}
Therefore, the interpretation under non-linear model could be decomposed into linear effect $\bm{l}(t)$ and non-linear effect $\bm{n}(t)$. And the linear effect could be decomposed as the inner product of $\bm{m}(t)$ and $\bm{\delta(\bm{f}(t))}$.
